# Supplementary material for: DSOL: A Fast Direct Sparse Odometry Scheme
Source: arXiv:2203.08182 source file (2022-03-15)
Supplement: Supplementary file 1 [file s80_appendix.tex]

\section{Appendix}

\subsection{Derivation of Direct Image Alignment}\label{sec:app/align}

\subsection{Derivation of Photometric Bundle Adjustment}\label{sec:app/adjust}

\subsection{Derivation of Frame Marginalization}\label{sec:app/marg}
